# Supplementary material for: On Robustness to $k$-wise Independence of Optimal Bayesian Mechanisms
Source: arXiv:2409.08547 source file (2024-09-13)
Supplement: Supplementary file 1 [file appendix0.tex]

In this appendix, we extend our result that the Myerson auction is pairwise-robust under identical regular distributions to non-regular distributions.

For non-regular margin $\dist$, we denote the corresponding regular distribution after ironing as $\distiron$. 
Denote the mutually independent joint distribution whose margins are them as $\distind$ and $\overline{\distind}$ respectively.
Recall that the item will be allocated to the bidder with the highest positive ironed virtual value in the Myerson auction for identical distributions.
If an interval is ironed, then the ironed virtual value in this interval will be the same.
According to Theorem 3.3.9 in \cite{hartline2013mechanism}, an allocation rule $x$ is optimal only if $x'(q) = 0$ when $q$ is in an ironed interval, which means that for each bidder, the probability that he is allocated when his value is in this interval will be the same\footnote{It should be noted that such allocation rule is not unique. When there is more than 1 bidder that has the largest virtual value, i.e., they are in the same ironed interval, there can be different tie-breaking rules, e.g., uniformly choosing one bidder or allocating to the bidder with the smallest index are all feasible rules.}. 
According to this observation and Myerson's lemma, if the winner's value is in an ironed interval, the payment of him will be the smallest value in this ironed interval, for both pairwise and mutually independent distributions. 
Thus if the quantile profile is fixed, the payment will be the same for $\dist$ and $\distiron$.

According to the argument above, our result for regular distribution can directly extend to non-regular distribution. Firstly, the Myerson auction can extract the same revenue from $\distind$ and $\overline{\distind}$. For each pairwise independent joint distribution $\dists$ whose margin is $\dist$, 
we can construct a corresponding $\overline{\dists}$ whose margin is $\distiron$ as follows: sample a random value vector $V$ follows $\dists$. Then we create another random value vector $\overline{V}$ where $\overline{V_i} = \distiron^{-1}(\dist(V_i))$, i.e., each dimension of $\overline{V}$ has the same quantile as which from $V$. $\overline{\dists}$ is the distribution which $\overline{V}$ follows.

From our construction, the Myerson auction gets the same revenue from $\dists$ and $\overline{\dists}$. Thus we have
\begin{equation*}
  c\cdot \Ex[\vals\sim\dists]{\Rev(\vals)} =  c\cdot\Ex[\vals\sim\overline{\dists}]{\Rev(\vals)}\geq \Ex[\vals\sim\overline{\distind}]{\Rev(\vals)} = \Ex[\vals\sim\distind]{\Rev(\vals)},
\end{equation*}
where $c$ is a constant smaller than 2.63, the inequality is due to our result for the regular case.
